# Supplementary material for: Occluded Human Mesh Recovery
Source: arXiv:2203.13349 source file (2022-03-24)
Supplement: Supplementary file 1 [file 6_qual_occlusion2.tex]

\begin{figure*}
 \captionsetup{font=small}
 \begin{center}

\includegraphics[height=0.16\textheight,width=0.48\linewidth]{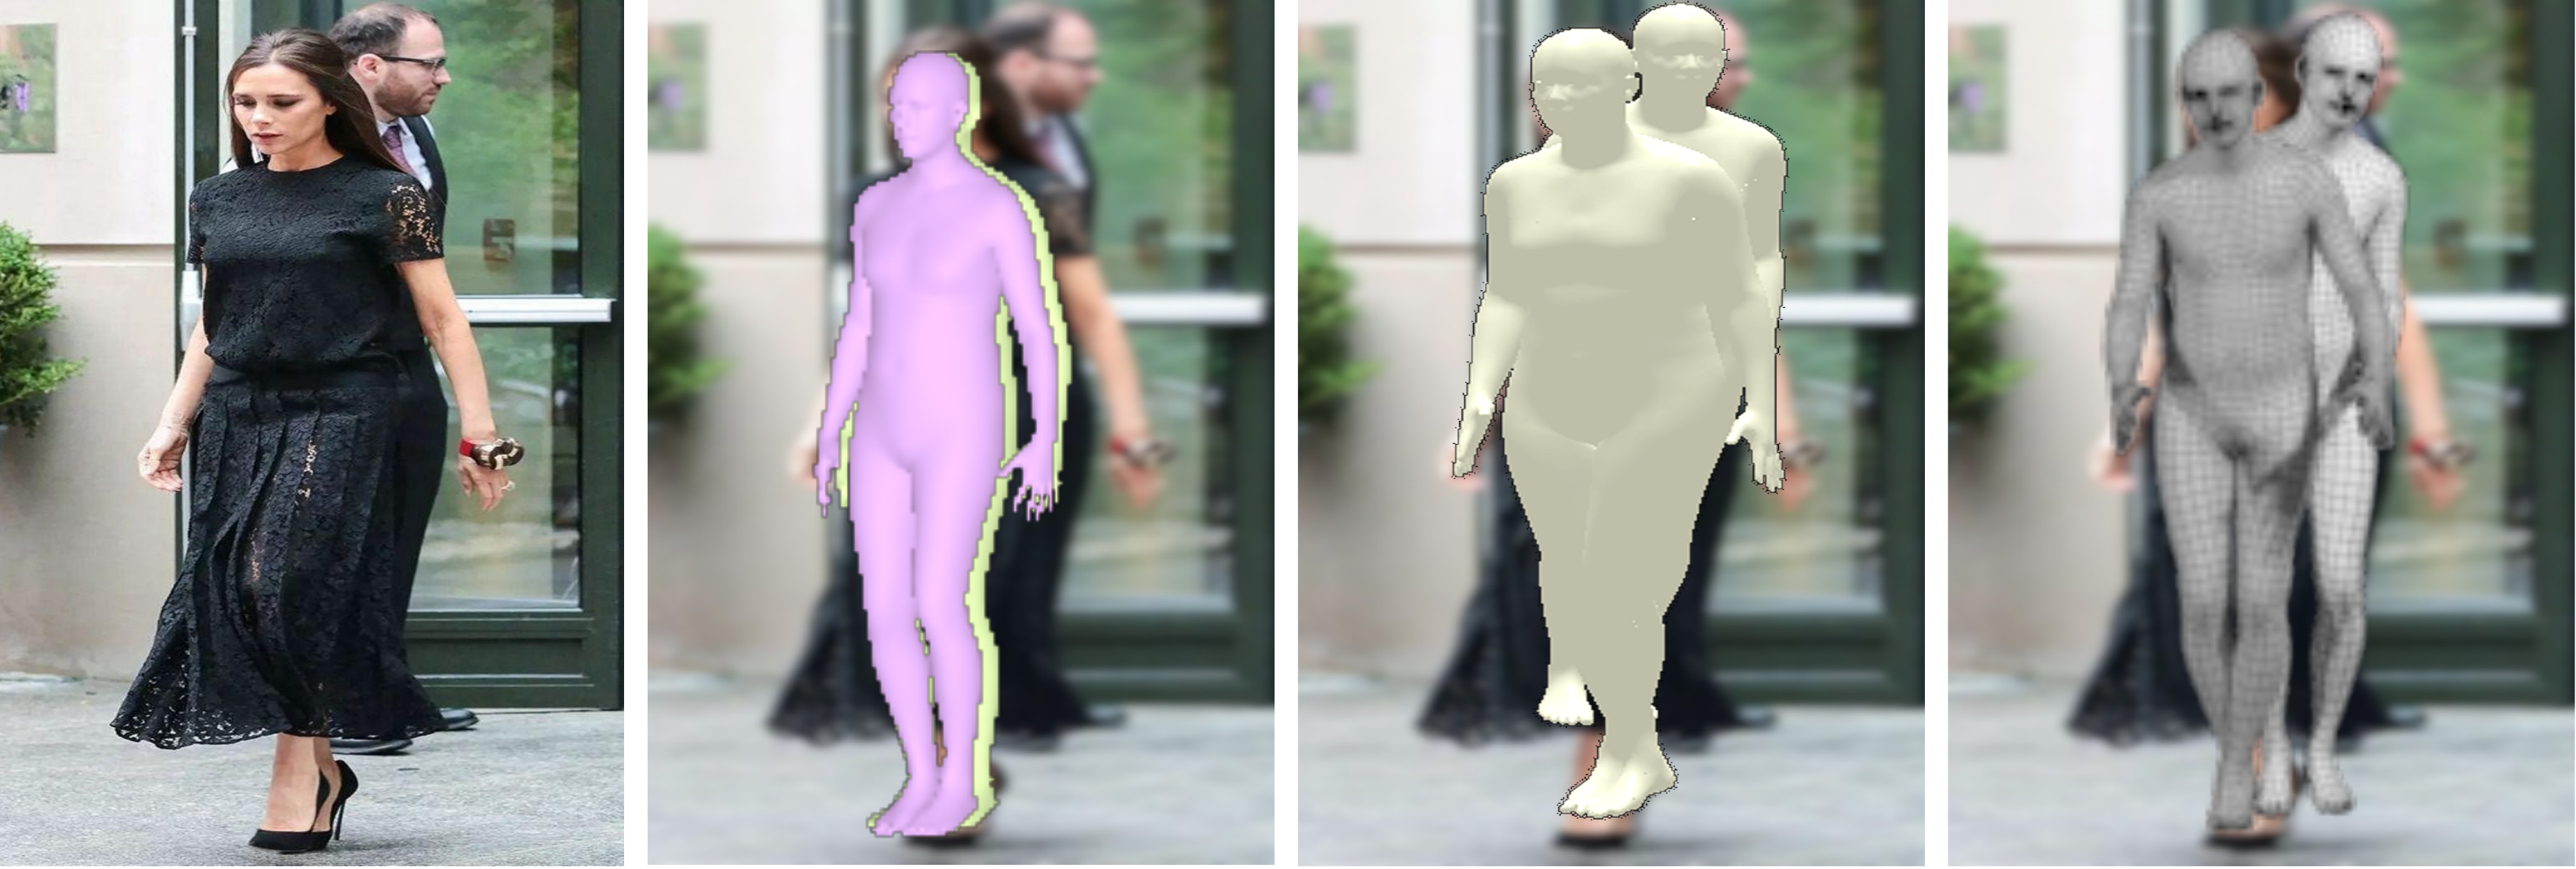}
\includegraphics[height=0.16\textheight,width=0.48\linewidth]{supplementary/images/occlusion1/01.pdf}

\includegraphics[height=0.16\textheight,width=0.48\linewidth]{supplementary/images/occlusion1/01.pdf}
\includegraphics[height=0.16\textheight,width=0.48\linewidth]{supplementary/images/occlusion1/01.pdf}

\includegraphics[height=0.16\textheight,width=0.48\linewidth]{supplementary/images/occlusion1/01.pdf}
\includegraphics[height=0.16\textheight,width=0.48\linewidth]{supplementary/images/occlusion1/01.pdf}

\includegraphics[height=0.16\textheight,width=0.48\linewidth]{supplementary/images/occlusion1/01.pdf}
\includegraphics[height=0.16\textheight,width=0.48\linewidth]{supplementary/images/occlusion1/01.pdf}

\includegraphics[height=0.16\textheight,width=0.48\linewidth]{supplementary/images/occlusion1/01.pdf}
\includegraphics[height=0.16\textheight,width=0.48\linewidth]{supplementary/images/occlusion1/01.pdf}

\includegraphics[height=0.16\textheight,width=0.48\linewidth]{supplementary/images/occlusion1/01.pdf}
\includegraphics[height=0.16\textheight,width=0.48\linewidth]{supplementary/images/occlusion1/01.pdf}

\end{center}
 \vspace*{-0.2in}
\caption{}
\label{figure:supplementary:qualitative1}
 \end{figure*}
